# Supplementary material for: DEPART: DEcomposing PARiTy across Multilingual LLMs
Source: arXiv:2605.28163 source file (2026-05-27)
Supplement: Supplementary file 1 [file appendix_deleted.tex]

\section{Per-language potential intervals}
\label{app:lp}

For each language $\ell$, the full model produces a posterior over the
``language potential'' $\mathrm{LP}_\ell$, the linear contribution
attributable to $\ell$ averaged over models and tasks:
\[
\mathrm{LP}_\ell \;=\; \mu + \boldsymbol{\gamma}^\top \mathbf{x}_\ell + \alpha_\ell.
\]
Table~\ref{tab:lp} reports the top-$10$ and bottom-$10$ languages by
posterior mean $\mathrm{LP}_\ell$ per bucket. The 90\% HDIs are wide
(approximately $1.9$--$2.2$ wide on the raw score scale), so
within-tier ranking should not be over-interpreted; the tier
membership (top vs.\ bottom) is the substantive read.

\begin{table*}[t]
\centering
\small
\setlength{\tabcolsep}{6pt}

\begin{tabular}{l l l}
\toprule
\textbf{Tier} &
\cellcolor{bucketNLU!55}\textbf{NLU} (top $\to$ bottom) &
\cellcolor{bucketReason!55}\textbf{Reasoning} (top $\to$ bottom) \\
\midrule
\textbf{Top 10}    & \texttt{nl(4), de(5), en(5), nb(4), sv(4),} & \texttt{ja(5), ar(5), eu(2), ko(4), tr(4),} \\
                   & \texttt{da(3), it(4), fr(5), es(5), ca(4)}  & \texttt{zh(5), kk(3), fr(5), hy(3), az(3)} \\
\midrule
\textbf{Bottom 10} & \texttt{gu(2), mr(2), te(1), kn(1), ml(1),} & \texttt{ta(3), bg(3), id(3), ml(1), af(3),} \\
                   & \texttt{sw(2), ta(3), wo(1), zu(2), or(1)}  & \texttt{is(2), zu(2), or(1), yo(2), wo(1)} \\
\bottomrule
\end{tabular}
\caption{Top-$10$ and bottom-$10$ languages by posterior mean
$\mathrm{LP}_\ell$ per bucket. Joshi class shown in parentheses.}
\label{tab:lp}
\end{table*}

\section{Full variance-share tables}
\label{app:variance}

Table~\ref{tab:variance} in the main text reports the posterior-mean
variance shares for NLU and Reasoning. Table~\ref{tab:variance_hdi}
below gives the same components with $90\%$ HDIs and adds the NLG
bucket.

\begin{table*}[t]
\centering
\small
\setlength{\tabcolsep}{6pt}

\begin{tabular}{l ccc}
\toprule
\textbf{Component} &
\cellcolor{bucketNLU!55}\textbf{NLU} &
\cellcolor{bucketReason!55}\textbf{Reasoning} &
\cellcolor{bucketNLG!55}\textbf{NLG} \\
\midrule
model                            & $66.7\%$ $[44.4, 87.2]$  & $12.7\%$ $[0.2, 40.0]$  & $33.8\%$ $[3.2, 81.3]$ \\
task $\times$ model              & $13.6\%$ $[5.0, 24.9]$   & $46.3\%$ $[25.9, 63.4]$ & $6.2\%$ $[0.6, 18.8]$ \\
model $\times$ language          & $6.9\%$ $[2.7, 11.3]$    & $9.4\%$ $[5.3, 14.0]$   & $1.1\%$ $[0.1, 3.4]$ \\
residual                         & $6.3\%$ $[2.5, 10.3]$    & $13.8\%$ $[8.4, 19.2]$  & $2.4\%$ $[0.3, 6.9]$ \\
task $\times$ language           & $3.6\%$ $[1.3, 6.2]$  & $4.3\%$  $[2.0, 7.3]$  & $0.1\%$  $[0.0, 0.4]$ \\
language residual                & $1.5\%$ $[0.0, 5.4]$  & $1.4\%$  $[0.0, 4.9]$  & $55.5\%$ $[0.7, 95.2]$ \\
fertility slope $\times$ model   & $1.4\%$ $[0.0, 6.1]$  & $12.1\%$ $[1.9, 33.7]$ & $0.8\%$  $[0.0, 3.7]$ \\
\bottomrule
\end{tabular}
\caption{Variance shares (posterior mean and $90\%$ HDI) per random
component in the full model, per bucket. Components sum to $100\%$ up
to MCMC noise.}
\label{tab:variance_hdi}
\end{table*}

\section{PPS, LDS, and MAVS --- definitions}
\label{app:pps_def}

For a set of cells $C$ (the entire bucket, or a per-model or
per-(model, benchmark) slice), the language-disparity share is the
fraction of total observed variance over the cells that is explained
by the language-varying components of the linear predictor:
\begin{equation}
\mathrm{LDS}_C \;=\; \frac{\mathrm{Var}_{c \in C}\!\bigl(\, \widehat{\eta}^{\mathrm{lang}}_c \,\bigr)}
                                  {\mathrm{Var}_{c \in C}\!\bigl(\, y_c \,\bigr)},
\end{equation}
where $\widehat{\eta}^{\mathrm{lang}}_c$ is the posterior expected
language-varying contribution at cell $c$, summing the language
fixed-effect terms, the categorical $\mathrm{script}/\mathrm{family}$
contributions, the language random intercept, and all interactions
involving language. MAVS uses the same denominator but a smaller
numerator: only the model-conditional measured features
\texttt{repr\_sim\_en} and \texttt{fertility} (with the per-model
random slope folded in):
\begin{equation}
\mathrm{MAVS}_C \;=\; \frac{\mathrm{Var}_{c \in C}\!\bigl(\, \gamma_{\mathrm{rs}} z^{\mathrm{rs}}_c + (\gamma_{\mathrm{f}} + r_{m(c)}) z^{\mathrm{f}}_c \,\bigr)}
                                   {\mathrm{Var}_{c \in C}\!\bigl(\, y_c \,\bigr)}.
\end{equation}
The ratio $\mathrm{MAVS}/\mathrm{LDS}$ is the fraction of the
language-attributable disparity that is captured by the
model-conditional measured features.

The parity-discounted score is
\begin{equation}
\mathrm{PPS}_5 \;=\; \overline{y}_C \;-\; 1.645 \cdot \sqrt{\mathrm{clip}(\mathrm{LDS}_C, 0, 1) \cdot \mathrm{Var}(y_C)},
\end{equation}
i.e.\ the mean score minus $1.645$ standard deviations of the
language-attributable noise. Under a Gaussian approximation,
$\mathrm{PPS}_5$ is the expected score on the language at the
$5$th percentile of difficulty for that model. We also report a
softer alternative,
$\mathrm{PPS}_w = \overline{y}_C \cdot (1 - \mathrm{clip}(\mathrm{LDS}_C, 0, 1))$,
in the supplementary CSVs.

\paragraph{Floor caveat.}
When a $(\mathrm{model}, \mathrm{benchmark})$ cell has near-constant
observed scores (within-cell SD $< 0.01$), the denominator in
$\mathrm{LDS}$ is tiny and the raw ratio exceeds $1$. We flag these
cells \texttt{floor\_cell=1} and clip $\mathrm{LDS}$ to $[0, 1]$
before computing $\mathrm{PPS}_5$. The raw $\mathrm{LDS}$ is preserved
in the supplementary CSVs for diagnostic use.

\section{Robustness check on the logit scale}
\label{app:robustness}

The full model uses a Gaussian likelihood on a $[0, 1]$ outcome, which
mis-specifies the boundary regime. We refit the full model with the
score replaced by $\mathrm{logit}(\text{score}_\epsilon)$ as a
robustness check. On NLU and Reasoning, all six continuous
coefficients retain their sign and credible-non-null classification;
the variance-share ordering is preserved within MCMC noise. Two
quantitative differences are worth noting: (i) the magnitude of
\texttt{repr\_sim\_en\_z} grows on the logit scale, consistent with
the bounded-Gaussian fit compressing the effect on the raw scale near
the high end of NLU scores; and (ii) the residual SD on Reasoning
drops from $0.065$ (raw) to $0.393$ (logit), which appears to enlarge
residual variance but in fact reflects the logit's stretching of the
$[0, 1]$ scale to $\mathbb{R}$ rather than a substantive worsening of
fit.

We caution that the logit-scale check does \emph{not} extend to the
two simpler model fits used to compute $R^2_{\text{ling}}$, which are
also Gaussian on the raw scale. The implicit defence is that
$R^2_{\text{ling}}$ is a ratio of $\sigma_\alpha^2$ values from two
fits on the same scale, so any compression artefact affects numerator
and denominator proportionally and largely cancels. On NLU and
Reasoning, where most scores live in the $0.3$--$0.8$ regime, this
defence is adequate. The NLG bucket (Section~\ref{app:nlg}), where
scores cluster near zero, is the case where the bounded-Gaussian
mis-specification could matter most --- but the NLG analysis is
already disqualified from $R^2_{\text{ling}}$ interpretation by
categorical sparsity, so the link-function issue is not the binding
constraint there. A fully principled alternative would replace the
Gaussian likelihood with a Beta or Binomial GLMM on all stages; we
defer this to future work.

\paragraph{Logit-scale robustness fit.}
Identical right-hand side to the full model, with the outcome replaced by
\[
\begin{aligned}
\text{score}_{\text{logit}} 
&= \log \frac{\text{score}_\epsilon}{1 - \text{score}_\epsilon} \\
\text{score}_\epsilon 
&= \mathrm{clip}(\text{score}, \epsilon, 1-\epsilon) \\
\epsilon 
&= 10^{-3}.
\end{aligned}
\]

\section{Sampling diagnostics}
\label{app:diagnostics}

Table~\ref{tab:diag} summarises convergence per bucket and per fit
(baseline, language-features, full model, logit robustness). For each
fit we flag whether the maximum $\hat{R}$ over all parameters and the
minimum bulk effective sample size meet the convergence thresholds
stated in the caption.

\begin{table*}[!ht]
\centering
\small
\setlength{\tabcolsep}{6pt}

\begin{tabular}{l l l l}
\toprule
\textbf{Fit} &
\cellcolor{bucketNLU!55}\textbf{NLU} &
\cellcolor{bucketReason!55}\textbf{Reasoning} &
\cellcolor{bucketNLG!55}\textbf{NLG} \\
\midrule
Baseline                  & OK                                  & OK                              & OK \\
Language-features         & WARN (script[Cyrillic] ESS $<100$)  & OK                              & OK \\
Full model                & WARN ($102$ params $\hat{R}>1.05$)  & OK (max $\hat{R} = 1.04$)       & OK (max $\hat{R} = 1.04$) \\
Logit robustness          & WARN ($4$ \texttt{C(task)} levels)  & OK (max $\hat{R} = 1.03$)       & WARN ($47$ params $\hat{R}>1.05$) \\
\bottomrule
\end{tabular}
\caption{Sampling diagnostics per fit per bucket. ``OK'' = all
$\hat{R}\le 1.05$ and min bulk ESS $\ge 100$; ``WARN'' flags at least
one parameter outside those thresholds (worst offender in
parentheses).}
\label{tab:diag}
\end{table*}

\paragraph{Where the warnings concentrate.}
The full-model warnings on NLU are concentrated on small-group random
intercepts: the $\mathrm{family}[\mathrm{Romance}/\mathrm{Uralic}/\mathrm{Germanic}/\mathrm{Slavic}]$
categorical levels (ESS in the $18$--$25$ range), the
$\sigma_\alpha$ hyperparameter itself (ESS $25$, $\hat{R} = 1.14$),
and several $\mathrm{task} \times \mathrm{model}$ cells with single-row
support. None of the substantive continuous coefficients
(\texttt{repr\_sim\_en\_z}, \texttt{joshi\_class\_z},
\texttt{fertility\_z}) have $\hat{R} > 1.04$, so the headline numbers
are not at risk. The convergence problems affect the per-script and
per-family fixed-effect contrasts, which we do not report in the main
text.

\paragraph{Remediation paths.}
Three options would address the NLU warnings: (i) increase warmup to
$10{,}000$ iterations, which is inexpensive on these graph sizes; (ii)
use a non-centred parameterisation for the language random intercept
and the script/family categoricals --- the canonical fix for divergent
sampling on small-group random effects with diffuse variance; or
(iii) pool sparse categorical levels into an ``Other'' bin (any
script or family with fewer than three languages in the frame). On
NLU, option (iii) would collapse approximately $13$ singletons. The
NLG logit-scale warnings are driven by \modelhl{famQwen}{Qwen-3.5-122B}'s
near-floor chrF, which under the logit transform produces a large
negative intercept that the sampler struggles to pin down; this is a
data issue (a generation pipeline anomaly specific to
\modelhl{famQwen}{Qwen-3.5-122B}) rather than a modelling one.

\begin{figure*}[t]
\centering
\begin{tikzpicture}
\begin{axis}[
    width=0.7\textwidth,
    height=7.2cm,
    xmin=-0.16, xmax=0.16,
    ymin=0.4, ymax=6.6,
    ytick={1,2,3,4,5,6},
    yticklabels={
        \texttt{repr\_sim\_en\_z},
        \texttt{fertility\_z},
        \texttt{geo\_dist\_en\_z},
        \texttt{phon\_dist\_en\_z},
        \texttt{syn\_dist\_en\_z},
        \texttt{joshi\_class\_z}
    },
    xtick={-0.15,-0.10,-0.05,0,0.05,0.10,0.15},
    xticklabel style={font=\small, /pgf/number format/fixed, /pgf/number format/precision=2},
    xlabel={Posterior coefficient (standardised score units)},
    xlabel style={yshift=-0.2em, font=\small},
    grid=major,
    grid style={dashed, gray!30},
    axis on top=false,
    before end axis/.code={
        \draw[black!60, line width=0.4pt] (axis cs:0,0.4) -- (axis cs:0,6.6);
    },
    legend pos=south east,
    legend cell align=left,
    legend style={
        font=\footnotesize,
        draw=none,
        fill=white,
        fill opacity=0.85,
        text opacity=1,
        at={(0.98,0.03)},
        anchor=south east
    },
    tick label style={font=\small},
    label style={font=\small},
    enlarge y limits=false,
]
% NLU
\addplot+[
    only marks,
    mark=*,
    mark size=2.2pt,
    color=black!85,
    error bars/.cd,
    x dir=both, x explicit,
    error bar style={black!85, line width=0.6pt},
] coordinates {
    ( 0.022, 1.18) +- (0.027, 0)
    (-0.012, 2.18) +- (0.033, 0)
    ( 0.009, 3.18) +- (0.013, 0)
    (-0.011, 4.18) +- (0.030, 0)
    (-0.021, 5.18) +- (0.029, 0)
    ( 0.065, 6.18) +- (0.014, 0)
};
\addlegendentry{NLU}
% Reasoning
\addplot+[
    only marks,
    mark=square*,
    mark size=2.0pt,
    color=red!70!black,
    error bars/.cd,
    x dir=both, x explicit,
    error bar style={red!70!black, line width=0.6pt},
] coordinates {
    ( 0.037, 0.82) +- (0.034, 0)
    ( 0.025, 1.82) +- (0.043, 0)
    ( 0.007, 2.82) +- (0.021, 0)
    (-0.007, 3.82) +- (0.037, 0)
    (-0.051, 4.82) +- (0.060, 0)
    ( 0.094, 5.82) +- (0.021, 0)
};
\addlegendentry{Reasoning}
\end{axis}
\end{tikzpicture}
\caption{Posterior means and $90\%$ HDIs for the six standardised
continuous predictors in the full model, per bucket.
\texttt{repr\_sim\_en\_z} is credibly positive (HDI excludes zero) in
both buckets; \texttt{joshi\_class\_z} reaches the threshold on
Reasoning. The remaining four predictors have HDIs that span zero,
reflecting absorption by the categorical script/family terms and the
language random intercept.}
\label{fig:forest}
\end{figure*}
